# Supplementary material for: Mechanised Assurance Cases with Integrated Formal Methods in Isabelle
Source: arXiv:1905.06192 source file (2019-05-15)
Supplement: Supplementary file 1 [file appendix.tex]

\section*{Tokeneer Model}
